# Supplementary material for: On some studies of Fraud Detection Pipeline and related issues from the scope of Ensemble Learning and Graph-based Learning
Source: arXiv:2205.04626 source file (2022-05-10)
Supplement: Supplementary file 1 [file appendix1.tex]

%!TEX root = ../thesis.tex
% ******************************* Thesis Appendix A ****************************
\chapter{How to install \LaTeX} 

\section*{Windows OS}

\subsection*{TeXLive package - full version}
\begin{enumerate}
\item	Download the TeXLive ISO (2.2GB) from\\
\href{https://www.tug.org/texlive/}{https://www.tug.org/texlive/}
\item	Download WinCDEmu (if you don't have a virtual drive) from \\
\href{http://wincdemu.sysprogs.org/download/}
{http://wincdemu.sysprogs.org/download/}
\item	To install Windows CD Emulator follow the instructions at\\
\href{http://wincdemu.sysprogs.org/tutorials/install/}
{http://wincdemu.sysprogs.org/tutorials/install/}
\item	Right click the iso and mount it using the WinCDEmu as shown in \\
\href{http://wincdemu.sysprogs.org/tutorials/mount/}{
http://wincdemu.sysprogs.org/tutorials/mount/}
\item	Open your virtual drive and run setup.pl
\end{enumerate}

or

\subsection*{Basic MikTeX - \TeX~ distribution}
\begin{enumerate}
\item	Download Basic-MiK\TeX (32bit or 64bit) from\\
\href{http://miktex.org/download}{http://miktex.org/download}
\item	Run the installer 
\item	To add a new package go to Start >> All Programs >> MikTex >> Maintenance (Admin) and choose Package Manager
\item	Select or search for packages to install
\end{enumerate}

\subsection*{TexStudio - \TeX~ editor}
\begin{enumerate}
\item	Download TexStudio from\\
\href{http://texstudio.sourceforge.net/\#downloads}
{http://texstudio.sourceforge.net/\#downloads} 
\item	Run the installer
\end{enumerate}

\section*{Mac OS X}
\subsection*{MacTeX - \TeX~ distribution}
\begin{enumerate}
\item	Download the file from\\
\href{https://www.tug.org/mactex/}{https://www.tug.org/mactex/}
\item	Extract and double click to run the installer. It does the entire configuration, sit back and relax.
\end{enumerate}

\subsection*{TexStudio - \TeX~ editor}
\begin{enumerate}
\item	Download TexStudio from\\
\href{http://texstudio.sourceforge.net/\#downloads}
{http://texstudio.sourceforge.net/\#downloads} 
\item	Extract and Start
\end{enumerate}

\section*{Unix/Linux}
\subsection*{TeXLive - \TeX~ distribution}
\subsubsection*{Getting the distribution:}
\begin{enumerate}
\item	TexLive can be downloaded from\\
\href{http://www.tug.org/texlive/acquire-netinstall.html}
{http://www.tug.org/texlive/acquire-netinstall.html}.
\item	TexLive is provided by most operating system you can use (rpm,apt-get or yum) to get TexLive distributions
\end{enumerate}

\subsubsection*{Installation}
\begin{enumerate}
\item	Mount the ISO file in the mnt directory
\begin{verbatim}
mount -t iso9660 -o ro,loop,noauto /your/texlive####.iso /mnt
\end{verbatim}

\item	Install wget on your OS (use rpm, apt-get or yum install)
\item	Run the installer script install-tl.
\begin{verbatim}
	cd /your/download/directory
	./install-tl
\end{verbatim}
\item	Enter command `i' for installation

\item	Post-Installation configuration:\\
\href{http://www.tug.org/texlive/doc/texlive-en/texlive-en.html\#x1-320003.4.1}
{http://www.tug.org/texlive/doc/texlive-en/texlive-en.html\#x1-320003.4.1} 
\item	Set the path for the directory of TexLive binaries in your .bashrc file
\end{enumerate}

\subsubsection*{For 32bit OS}
For Bourne-compatible shells such as bash, and using Intel x86 GNU/Linux and a default directory setup as an example, the file to edit might be \begin{verbatim}
edit $~/.bashrc file and add following lines
PATH=/usr/local/texlive/2011/bin/i386-linux:$PATH; 
export PATH 
MANPATH=/usr/local/texlive/2011/texmf/doc/man:$MANPATH;
export MANPATH 
INFOPATH=/usr/local/texlive/2011/texmf/doc/info:$INFOPATH;
export INFOPATH
\end{verbatim}
\subsubsection*{For 64bit OS}
\begin{verbatim}
edit $~/.bashrc file and add following lines
PATH=/usr/local/texlive/2011/bin/x86_64-linux:$PATH;
export PATH 
MANPATH=/usr/local/texlive/2011/texmf/doc/man:$MANPATH;
export MANPATH 
INFOPATH=/usr/local/texlive/2011/texmf/doc/info:$INFOPATH;
export INFOPATH

\end{verbatim}

%\subsection{Installing directly using Linux packages} 
\subsubsection*{Fedora/RedHat/CentOS:}
\begin{verbatim} 
sudo yum install texlive 
sudo yum install psutils 
\end{verbatim}

\subsubsection*{SUSE:}
\begin{verbatim}
sudo zypper install texlive
\end{verbatim}

\subsubsection*{Debian/Ubuntu:}
\begin{verbatim} 
sudo apt-get install texlive texlive-latex-extra 
sudo apt-get install psutils
\end{verbatim}
